# Supplementary material for: Freditor: High-Fidelity and Transferable NeRF Editing by Frequency Decomposition
Source: arXiv:2404.02514 source file (2024-04-03)
Supplement: Supplementary file 1 [file 07_appendix_0.tex]

\section{Structure of Supplementary Material}
Our supplementary material includes the following contents:

$\bullet$ A theoretical proof of edits on low-frequency components yields higher multi-view consistency than edits on full images.

$\bullet$ Details of training, including network parameters and training setting.
 
% $\bullet$ More analysis to inspect where the blur on edited 3D scenes comes from.

$\bullet$ Further visualization of our method on high-fidelity, transferable editing and intensity control.
